# Supplementary material for: Deep Closest Point: Learning Representations for Point Cloud Registration
Source: arXiv:1905.03304 source file (2019-05-08)
Supplement: Supplementary file 1 [file supplement.tex]

\section*{Supplementary Material}

\subsection*{Code}
We release our code anonymously \url{https://drive.google.com/open?id=1xaSYdVXB4WEfWOazCGckuYSANQovjK4C} along with pretrained DCP-v1 and DCP-v2.
\subsection*{Details of the Model}
Both DCP-v1 and DCP-v2 use DGCNN to embed point clouds. In DGCNN, we use five EdgeConv layers. The numbers of filters per layer are $[64, 64, 128, 256, 512]$. In each EdgeConv layer, BatchNorm is used \cite{Ioffe2015} with 0.1 momentum, followed by ReLU \cite{Nair2010}. Following \cite{dgcnn}, we concatenate the outputs from the first four layers and feed them into the last one. Our local aggregation function is $\max$, and no global aggregation function is needed. 

For DCP-v2, in the Transformer layer, the architecture is the same as the one proposed in \cite{Vaswani2017}.  The only difference is that we do not add positional encoding, because the position of each point in $\R^3$ is not correlated with its index in the array.

We use one encoder and one decoder. In both the encoder and decoder, we use multi-head attention with 4 heads and 512 embedding dimensions, followed by a MLP with 1024 hidden dimensions. ReLU \cite{Nair2010} is also used in the MLP. Inside the Transformer, LayerNorm \cite{layernorm} is used after MLP and multi-head attention and before the residual connection. Unlike \cite{Vaswani2017}, we do not use Dropout \cite{dropout}. 

We use PyTorch's \cite{paszke2017automatic} built-in SVD layer. Other numerical solvers that support gradient backpropagation could also be used to recover the rigid transformation. 

Adam \cite{KingmaB14} with initial learning rate 0.001 is used for training. The coefficients used for computing running averages of the gradient and its square are 0.9 and 0.999, resp. 

We use weight decay $10^{-4}$ to regularize the model. We train the model a total of 250 epochs, and at epochs 75, 150 and 200, the learning rate is divided by 10. 

The MLP we use in ablation study has 3 fully connected layers and the number of filters are $[256, 128, 64]$ respectively. BatchNorm \cite{KingmaB14} and ReLU \cite{Nair2010} are used after each fully connected layer. Finally, another two fully connected layers are used to project the embeddings to quaternion and translation vector separately.

The architecture of PointNet in ablation study is the same as the basic version in \cite{QiSMG17}. The number of filters in each layer are $[64, 64, 64, 128, 512]$.

\subsection*{Additional Figures}
\vskip 0.1in
\begin{figure*}[t!] 
  \centering
 \includegraphics[width=2.0\columnwidth]{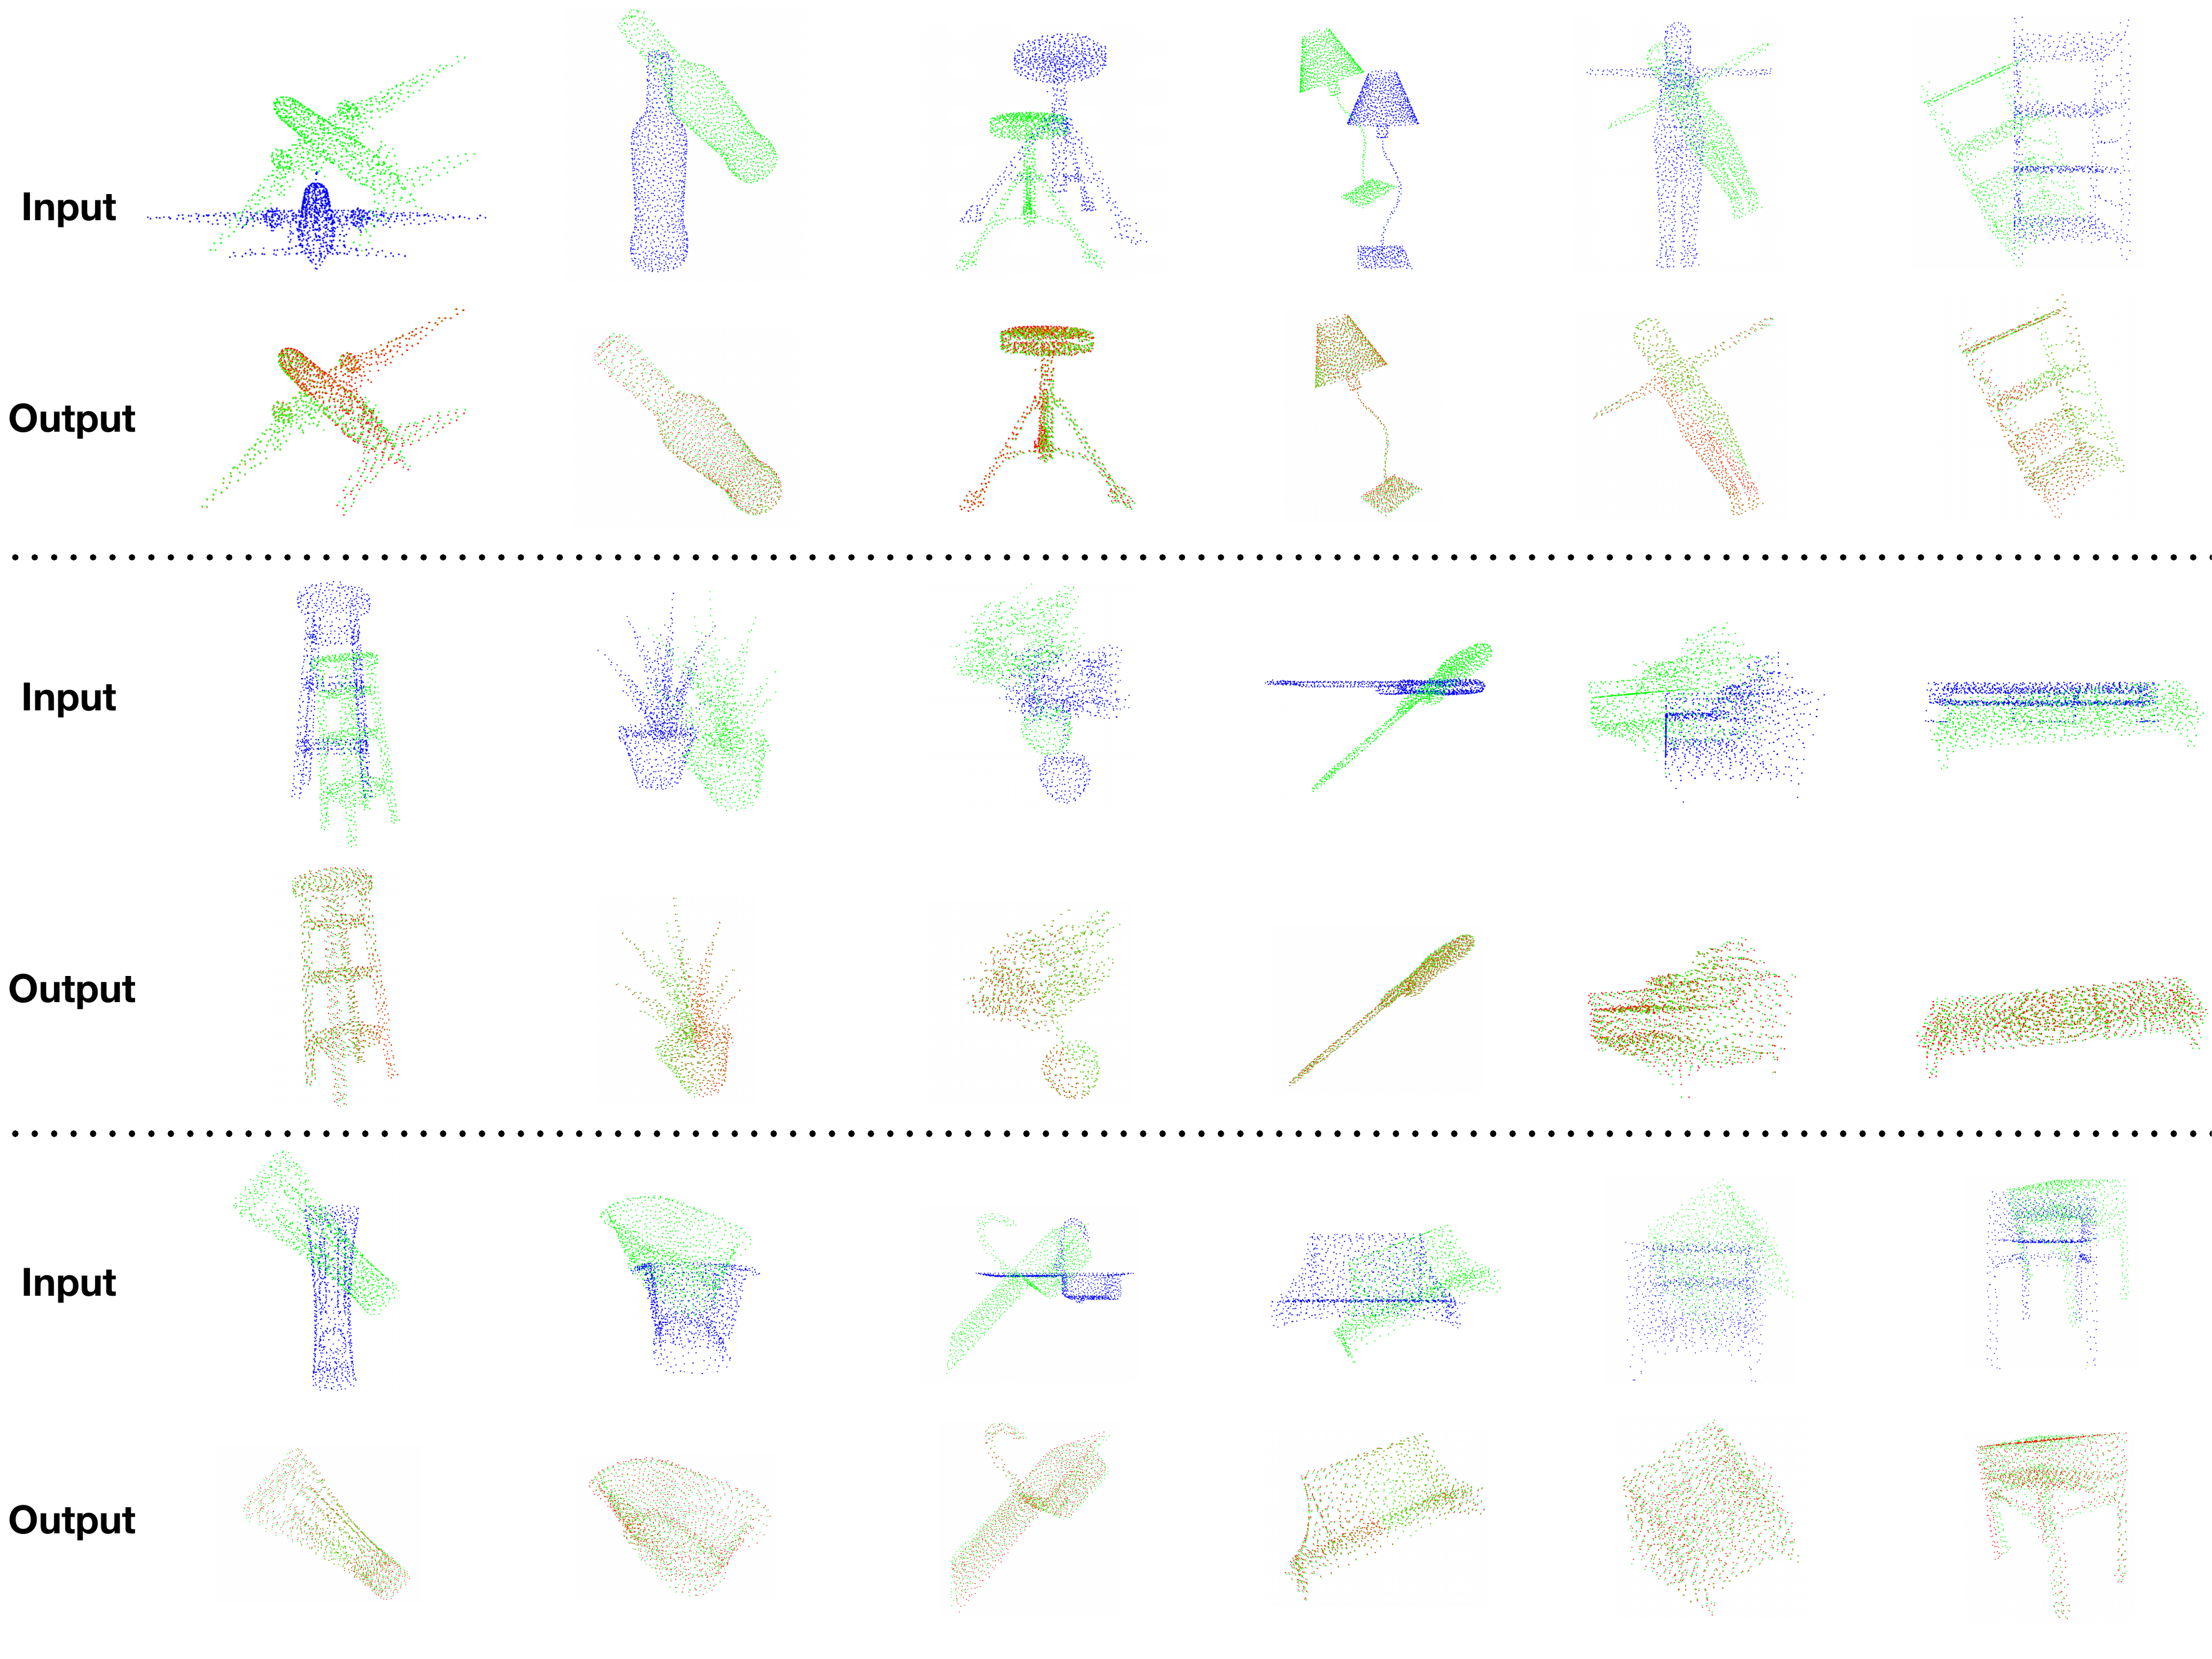}
  \caption{Results of DCP-v2. \textbf{Top}: inputs. \textbf{Bottom}: outputs of DCP-v2.  \label{fig:moreplot}}
\vskip 0.1in
\end{figure*}

We provide additional figures of results with DCP-v2 tested on different objects in Figure \ref{fig:moreplot}. Figure \ref{fig:largemotion} shows results in which we test with rotations in all of $\SE(3)$, meaning along each axis, we randomly sample rotations in $[0, 360^\circ]$. The model used here is still trained with rotations in $[0, 45^\circ]$. As shown in Figure \ref{fig:largemotion}, our model generalizes reasonably well to large motions. Figure \ref{fig:noise} shows the results of DCP-v2 tested on noisy point clouds. The noises (sampled from $\mathcal{N}(0, 0.01)$) are added independently to each point of two input point clouds. 

\begin{figure*}[t!] 
  \centering
  \vskip -0.5in
 \includegraphics[width=2.0\columnwidth]{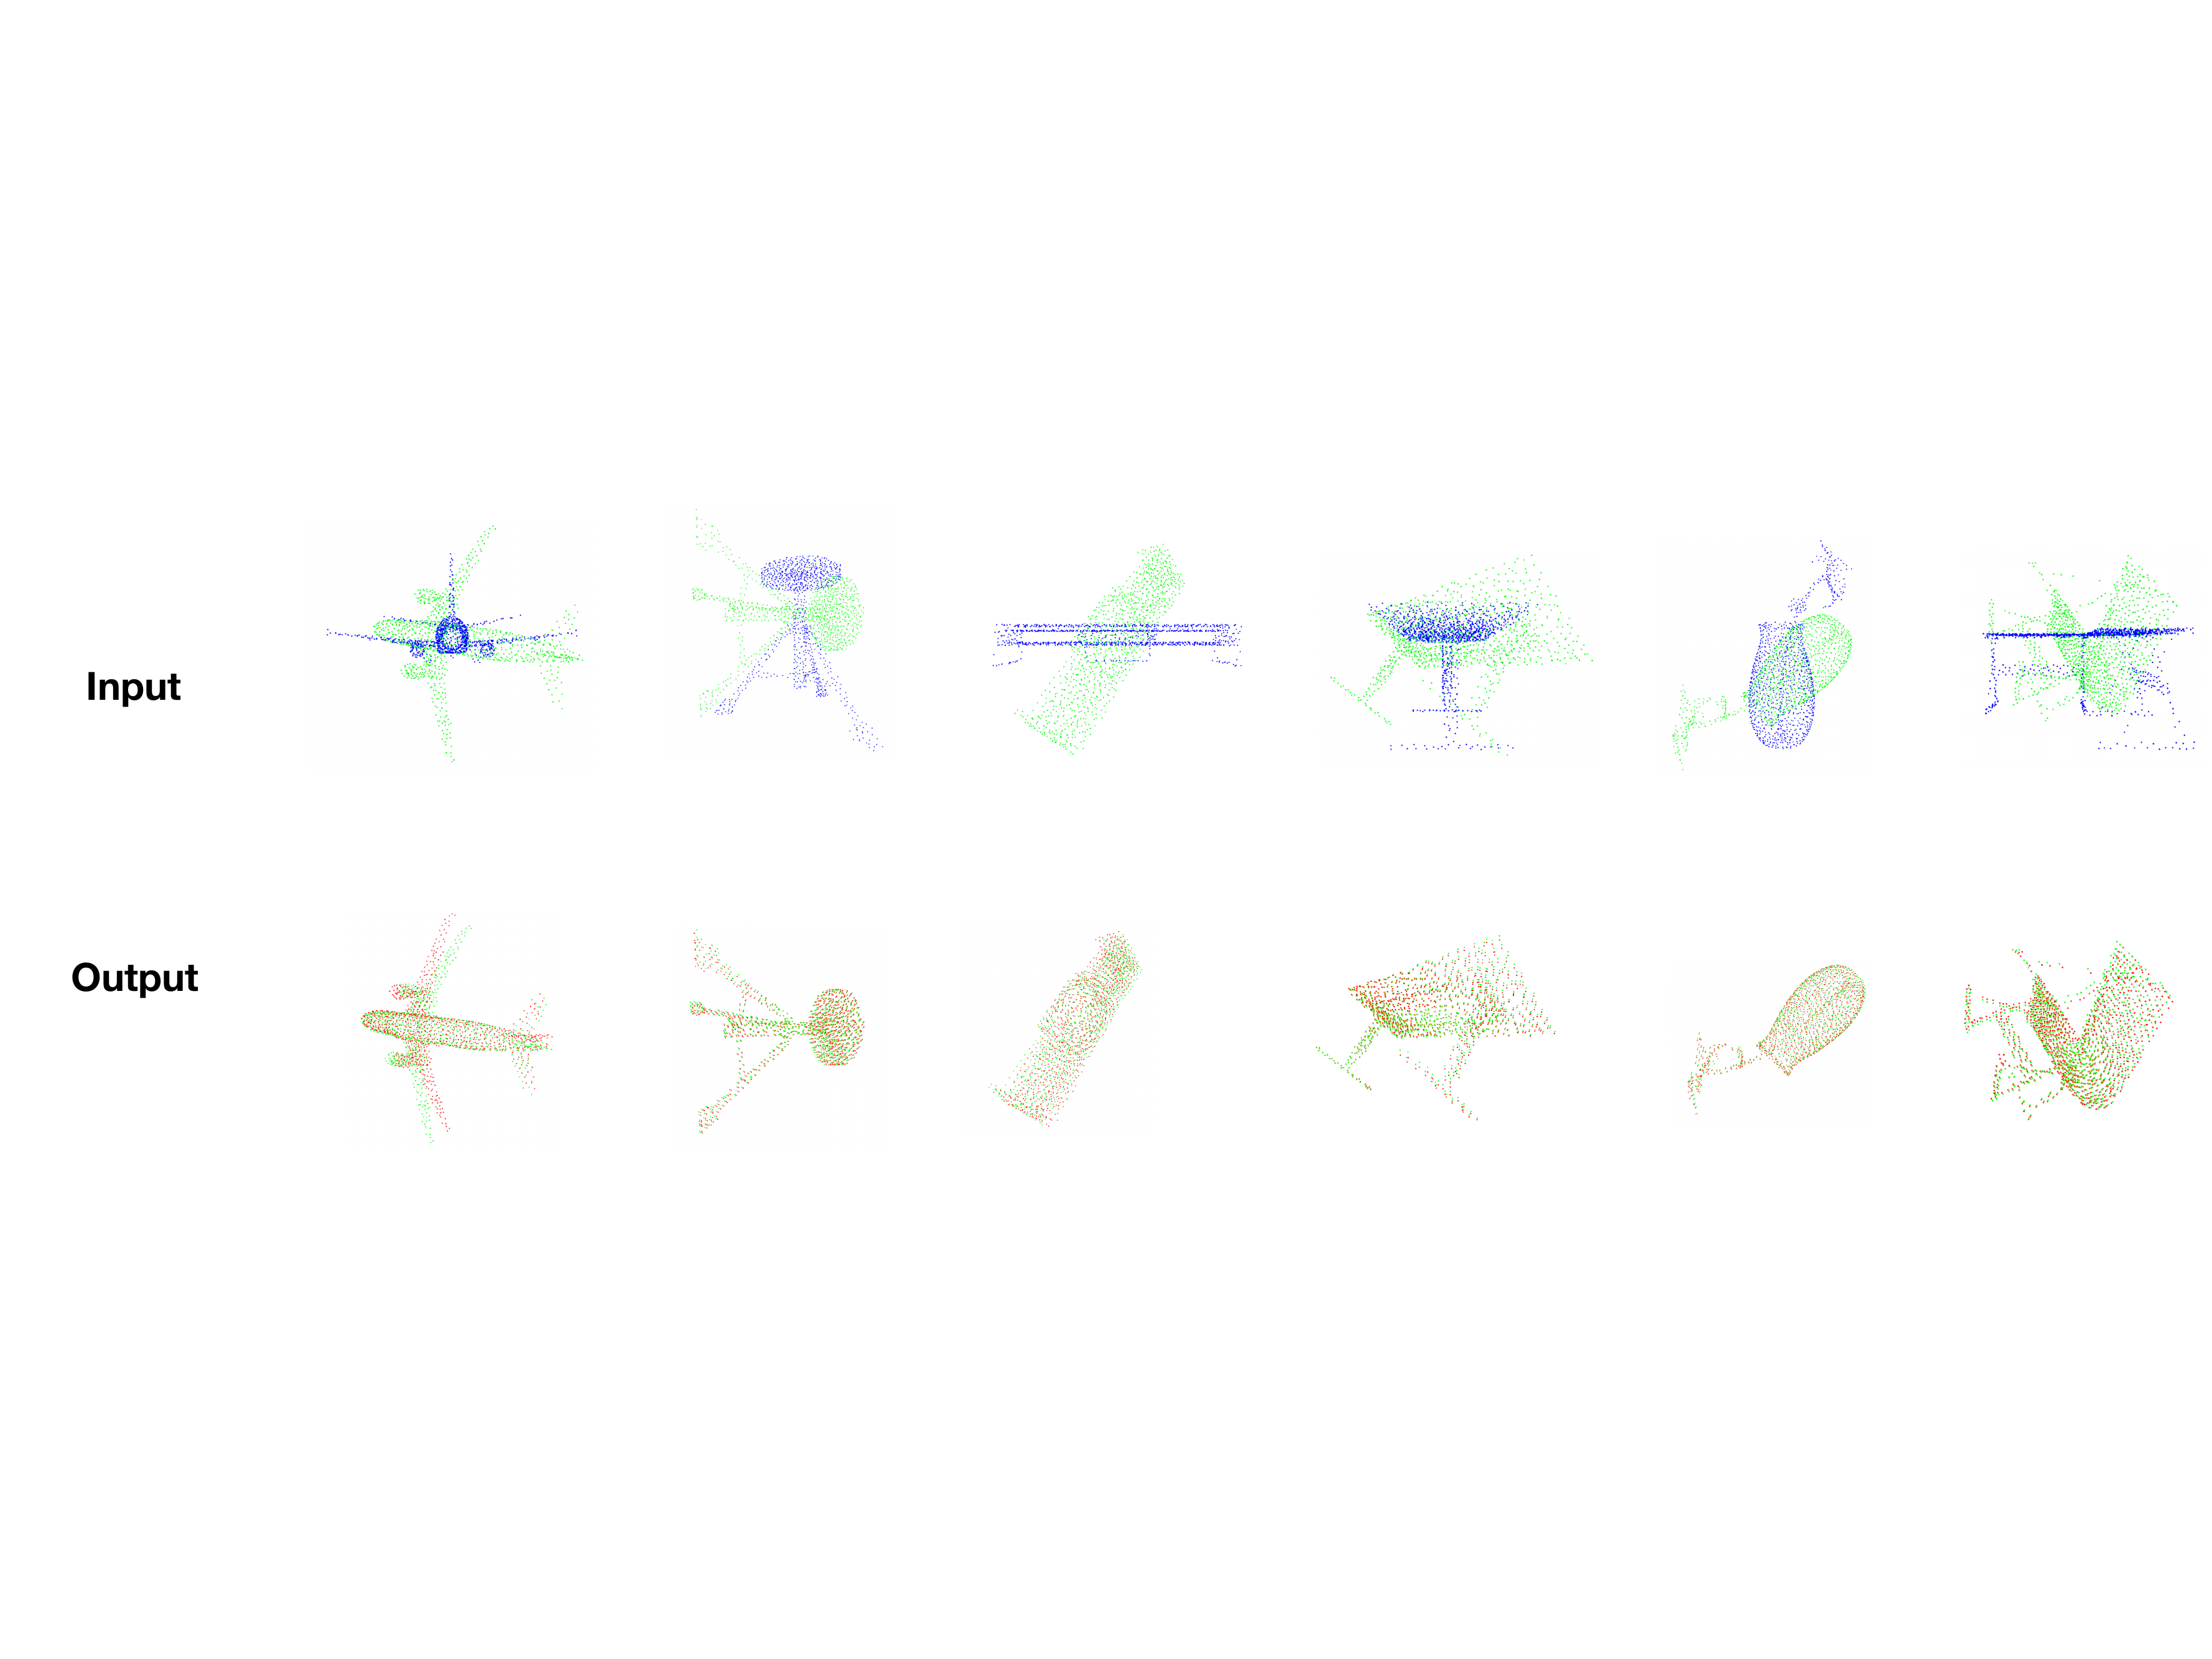}
 \vskip -1.0in
  \caption{Results of DCP-v2 tested with large motion. \textbf{Top}: inputs. \textbf{Down}: outputs of DCP-v2  \label{fig:largemotion}}
\end{figure*}

\begin{figure*}[t!] 
  \centering
 \includegraphics[width=2.0\columnwidth]{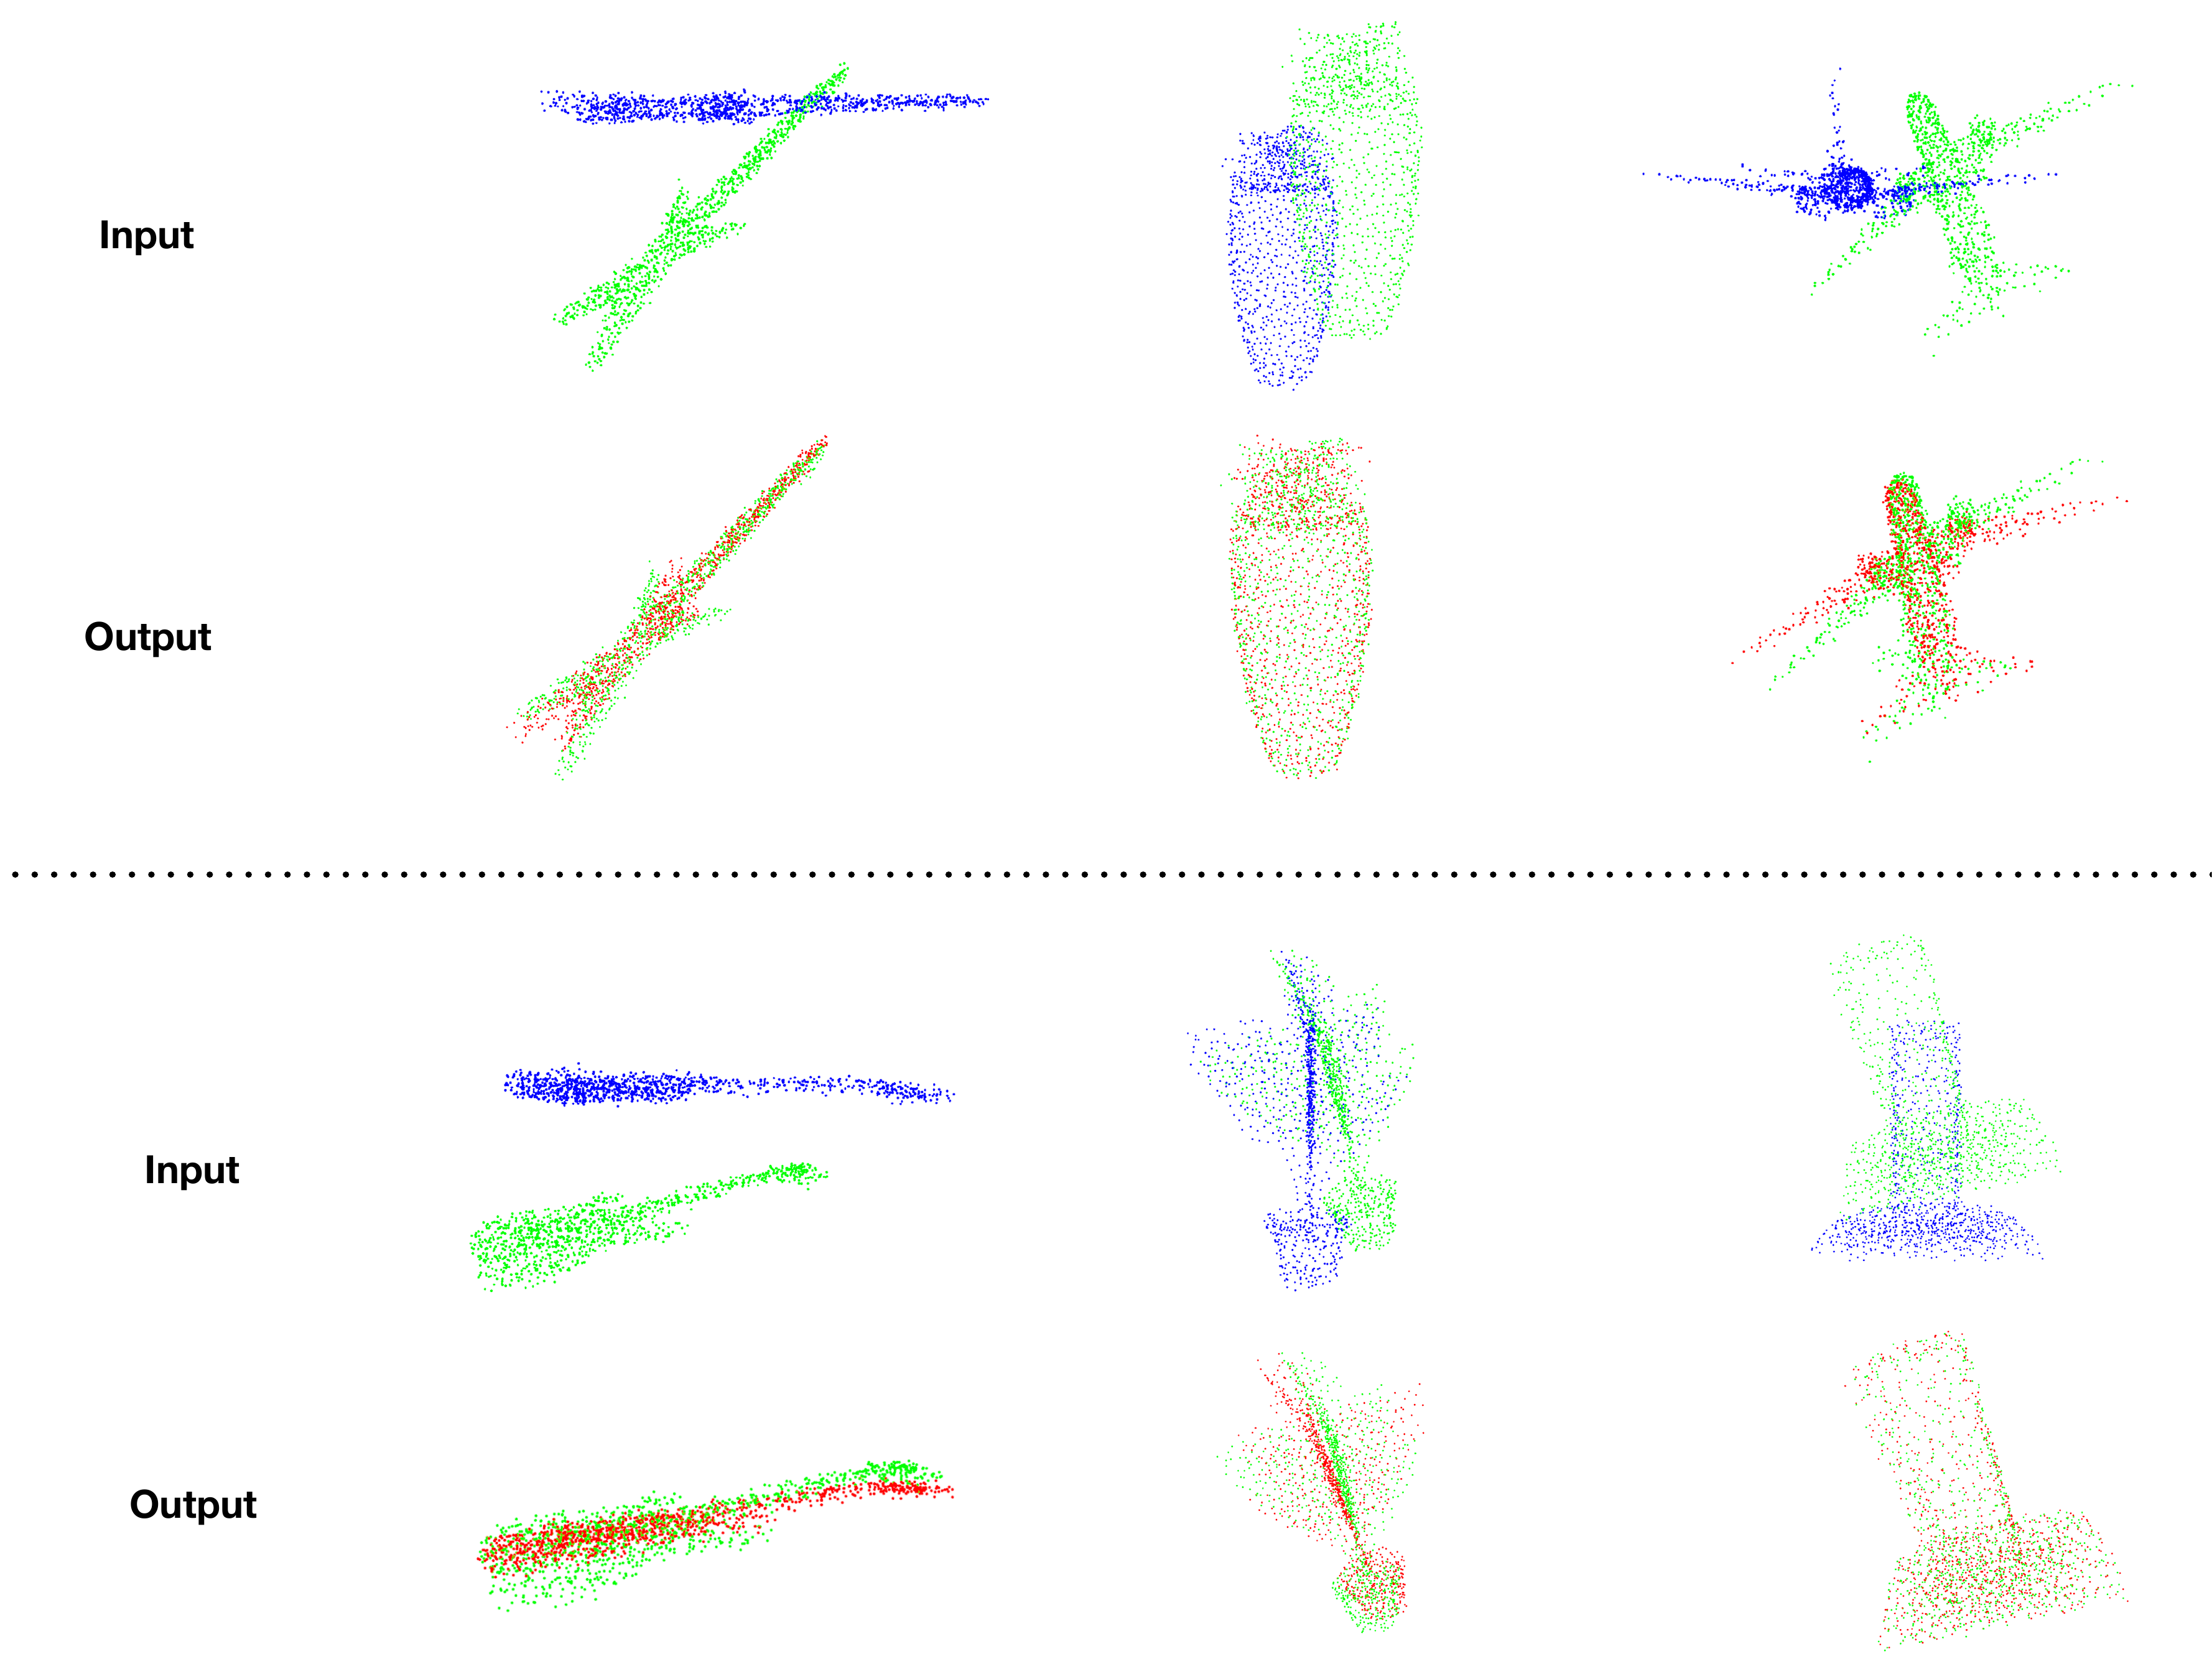}
  \caption{Results of DCP-v2 tested on noisy point clouds. \textbf{Top}: inputs. \textbf{Down}: outputs of DCP-v2  \label{fig:noise}}
\end{figure*}
